# Supplementary material for: CodedVO: Coded Visual Odometry
Source: arXiv:2407.18240 source file (2024-07-25)
Supplement: Supplementary file 1 [file supp.tex]

\subsection{Abalation Study}
\subsubsection{Effect of different phase mask sizes}

\begin{table}[H]
\centering
\label{table:size_ablation}
\begin{tabular}{l|ccc|c}
\toprule
\textbf{Size} & \textbf{L1} & \textbf{L1 under 3m} & \textbf{RMSE} & \textbf{ATE} \\
\midrule
$11 \times 11$ & 0.157 & 0.133 & 0.210 \\
$51 \times 51$ &0.142 & 0.117 & 0.195  \\
\midrule
$23 \times 23$ (Ours) & 0.133 & 0.177 & 0.197 & 0.12  \\
\bottomrule
\end{tabular}
\caption{Depth estimation \& VO ATE errors for different phase mask sizes for ICL-NUIM\cite{handa:etal:ICRA2014}, Living Room Traj1 (lr-kt1)}
\end{table}
\subsubsection{Effect of different focus distances}

\begin{table}[H]
\centering
\label{table:focus_ablation}
\begin{tabular}{l|ccc|c}
\toprule
\textbf{Focus Distance} & \textbf{L1} & \textbf{L1 under 3m} & \textbf{RMSE} & \textbf{ATE} \\
\midrule
50 cm  & 0.175 & 0.153 & 0.233 \\
250 cm & 0.111 & 0.094 & 0.169 \\
\midrule
85 cm (Ours) & 0.133 & 0.177 & 0.197 & 0.12 \\
\bottomrule
\end{tabular}
\caption{Depth estimation \& VO ATE errors for different focus distances for ICL-NUIM\cite{handa:etal:ICRA2014}, Living Room Traj1 (lr-kt1)}
\end{table}
\section{Conclusion and Discussion}
\label{sec:conclusion}
\subsection{Limitations}

\section{Summary of the paper}
\begin{itemize}
    \item Exploring what constraints can non-circular apertures in cameras can bring to improve estimations in robotics.
    % \item In this work, we would be exploring few things:
    % \begin{itemize}
        % \item Major focus: Visual Odometry (Pose Estimation)
        % \item 3D Flow / Optical Flow
        % \item SLAM/SfM
    % \end{itemize}
    % \item Exploring learning depth from aperture masks (all in simulation) (If we work on real world, it will only be amplitude masks): 
    % \begin{itemize}
        % \item Amplitude Masks
        % \item Phase Masks
        % \item Fisher Masks
    % \end{itemize}
    \item Major known issues:
    \begin{itemize}
        % \item Due to the unknown scale factor, methods are benchmarked by optimizing the scale with the ground truth maps for measuring odometry accuracy. 
        % \item No dataset exists. Will require to train and test using data from the same sensor to simulate metric depth estimation. No need to talk about Generalization.
        % \item We need to compare our work with MiDasv3 (that offers metric depth estimation). Hopefully we are better at least in terms of `metric' error. Visually it can be better.
        \item While recovering RGB images from the `coded blurred image' creates artifacts which are not consistent over frames which hinders the performance of feature matching. It will not be a big deal for visual odometry since most methods work on bluring the images for feature matching. It might be a problem for flow and structure from motion problems.
    \end{itemize}
\end{itemize}

% \section*{Plausible contributions}
% \begin{itemize}
    % \item Check if MiDasv3.1 metric depth estimation is consistent across frames. This method will be our major comparison methods for `RGB-D' VO method. Ideally, we need to be better than MiDaSv3.1 is some way so we have an argument. Either metric consistency over frames, speed of depth computation and/or accuracy of metric depth itself (maybe all 3 of above).
    % \item Comparison of metric depth error using amplitude, phase and Fisher masks and their results on the same VO methods on a two test sets (one in-domain and one out-of-domain) - both visual and metric error.
    % \item Comparison of error in pose estimation (in the data mentioned above) - both visual and metric error.
    % \item Comparison of error in 3D Flow estimation (in the data mentioned above) - both visual and metric error.
    % \item Real world experiments (if time persists) for amplitude masks.
    % \item Most likely for next paper: Comparison of error in SfM (in the data mentioned above) - both visual and metric error.
    % Note: All our experiments will be performed on one or two RGB-D VO methods only and will be compared with all the standard and state-of-the-art RGB VO methods. 
% \end{itemize}

\begin{itemize}
    % \item What is the problem that exists?
    % \item Why are we doing this?
    % \item Have researchers/industry done something to approach/solve this problem in the past?
    % \item What are we doing? How are we approaching the problem?
    % \item How will this solve this problem?
    \item Assumptions?
    % \item How efficient/``good'' is the solution?
    % \item How will it solve the issues?
    \item What are the drawbacks of this approach?
    \item Future Work?
\end{itemize}

% References are important to the reader; therefore, each citation must be complete and correct. If at all possible, references should be commonly available publications.
